# Supplementary material for: Social Network Integration: Towards Constructing the Social Graph
Source: arXiv:1311.2670 source file (2014-01-21)
Supplement: Supplementary file 1 [file appendix.tex]

\section{Appendix: Feature Definitions}
\label{sec:appendix}

%In this section 
Table \ref{tb:feature} summarizes how we define the factor functions in our experiments. 
%We total define thirteen pairwise factor features and two types of correlation factor functions. Table \ref{tb:feature} give a summary of local feature definitions.

\begin{table}[h]
\centering \caption{\label{tb:feature} Features defined for co-invention relationship $(v_i, v_q)$.}
\small
\newcommand{\minitab}[2][l]{\begin{tabular}{#1}#2\end{tabular}}
\begin{tabular}{@{  }c|p{5.9cm}}
\hline
\textbf{Feature} & \textbf{Description} \\ \hline
\#Patent & Number of patents published by $v_i$\\ \hline
\#Co-inventor & Number of existing co-inventors of $v_i$\\ \hline
Ratio & \#Patent / \#Collaborator\\ \hline
Experience & Difference of the years of the first patent published by $v_q$ and $v_i$ \\ \hline
CS-interest & Cosine similarity of interests between $v_q$ and $v_i$ \\ \hline
\#C-interests & Number of common interests between $v_q$ and $v_i$ \\ \hline
\#P-interests & Percentage of common interests between $v_q$ and $v_i$ \\ \hline
%Average percentage & average percentage of common research interests of $v_q$ and $v_i$ \\ \hline
Cat-similarity & Similarity between patents' categories of $v_q$ and $v_i$ \\ \hline

\#C-neighbor & Number of common co-inventors of $v_q$ and $v_i$\\ \hline
\#2-C-neighbor & Number of 2-step common co-inventors of $v_i$ and $v_j$\\ \hline

Referral & Referral chaining length between $v_q$ and $v_i$ \\ \hline
Recency & Difference of current year and last collaborated year between $v_q$ and $v_i$ over the referral chaining\\ \hline 

Correlation & Represent whether two candidates have a co-invention relationship. \\ \hline
%Structural hole correlation & If two candidates have a collaboration and one of them is structural hole, then define a Structural hole correlation feature. \\ \hline
\end{tabular}
\normalsize
\end{table}

\hide{
In this section we introduce how we define the factor functions in our experiments. We total define nine pairwise factor features which can divide into three categories: Status homophily, Link homophily, and Research homophily. %, Geographic distance.
In addition, we also define two types of correlation factor functions.

\vpara{Status homophily} From our database, we extract some useful statues of inventors, including patent number of inventors and candidates, the number of collaborators, interests and personal patents published year. Based on these five values, we define the following four features: patent number, collaborator number, first patent published interpolation,  similarity of interests between inventors and candidates.

\vpara{Link homophily} We create undirected edges between users and candidates using collaborated patents, and define the number of common neighbors of them as a feature.and define the following feature: the number of neighbors between two user.

\vpara{Research homophily} We consider the research homophily between users and candidates and define the following four features: the number of common research interests, percentage of common research interests of each user and the average percentage.

\vpara{Directed correlation} For each query user and candidates, we create a pairwise node in the factor graph. When two candidates have a collaboration, we then define a directed correlation feature.

\vpara{Structural hole correlation} For each query user and candidates, we create a pairwise node in the factor graph. When two candidates have a collaboration and one of them is structural hole, we then define a Structural hole correlation feature.
\hide{
\vpara{Geographic distance} We use Arnetminer.org to get the address of candidates and users. We define whether or not the users and candidates come from the same country as a feature.
}

%\para{Structural balance}  Based on the structural balance theory, we define four features representing all situations of structural balance theory for each triad.
\hide{
\begin{table}[t]
\centering \caption{\label{tb:aufeature} Features defined for edge $(v_i, v_j)$ in Coauthor. \small $P_i$ denotes a set of papers published by author $v_i$.  \small $C_i$ denotes a set of authors who collaborate with $v_i$. \normalsize}
\centering
\small
\newcommand{\minitab}[2][l]{\begin{tabular}{#1}#2\end{tabular}}
\begin{tabular}{c||p{5cm}}
\hline
Feature & Description \\ \hline
\#Paper & $|P_i|$, $|P_j|$ \\ \hline
Paper Ratio & $|P_i|/|P_j|$ \\ \hline
Coauthor Ratio & $|P_i \cap P_j|/|P_i|$, $|P_i \cap P_j|/|P_j|$ \\ \hline
\#Common Coauthor & $|C_i \cap C_j|$ \\ \hline
\minitab[c]{Common Coauthor\\Ratio} & $|C_i \cap C_j|/|C_i|$, $|C_i \cap C_j|/|C_j|$ \\ \hline
H-index Diff & The difference in H-index of $v_i$ and $v_j$ \\ \hline
\minitab[c]{First-pub-year\\Diff} & The difference in year of  the first earliest publication of $v_i$ and $v_j$ \\ \hline
Distance Correlation & Social distance of $v_i$ and $v_j$ \\ \hline
%Max. Flow & The max flow between $v_i$ and $v_j$ \\ \hline
\end{tabular}
\normalsize
\end{table}
}

\begin{table}[t]
\centering \caption{\label{tb:pafeature} Features defined for edge $(v_i, v_j)$ in Coworker.}
\centering
\small
\newcommand{\minitab}[2][l]{\begin{tabular}{#1}#2\end{tabular}}
\begin{tabular}{c||p{5cm}}
\hline
Feature & Description \\ \hline
Volume & $|P_i|/|C_i|$, $|P_j|/|C_j|$ \\ \hline
Degree & $|C_i|$, $|C_j|$ \\ \hline
\#Patent & $|P_i|$, $|P_j|$ \\ \hline
Cosine Similarity & We generate vector $\mathbf{w_i}$,$\mathbf{w_j}$ with patent categories, then apply $$Sim(\mathbf{v_i}, \mathbf{v_j}) = \frac{\mathbf{w_i}\cdot\mathbf{w_j}}{||\mathbf{w_i}||||\mathbf{w_j}||}$$ \\ \hline
\#Common Coauthor & $|C_i \cap C_j|$ \\ \hline
Distance Correlation & Social distance of $v_i$ and $v_j$ \\ \hline
Age Similarity & Age difference approximated by the difference of the year of the first patent published by the two inventors \\ \hline
\end{tabular}
\normalsize
\end{table}
}
